# Supplementary material for: Combinatorial Rising Bandits
Source: arXiv:2412.00798 source file (2026-03-03)
Supplement: Supplementary file 1 [file heatmap4_appendix.tex]

\begin{figure}[!ht]
\centering
    \begin{subfigure}{0.06\linewidth}
        \rotatebox{90}{500}
        \vspace{1.2cm}
        \vfill
        \rotatebox{90}{1500}
        \vspace{1.3cm}
        \vfill
        \rotatebox{90}{3000}
        \vspace{1.1cm}
    \end{subfigure}
    \hspace{-0.7cm}
    \begin{subfigure}{0.133\linewidth}
        \centering
            \includegraphics[width=0.98\linewidth, trim={3.2cm 1cm 3.2cm 1cm},clip]{./figure/images/heatmap6_optimal_500-n.pdf}
            \includegraphics[width=0.98\linewidth, trim={3.2cm 1cm 3.2cm 1cm},clip]{./figure/images/heatmap6_optimal_1500-n.pdf}
            \includegraphics[width=0.98\linewidth, trim={3.2cm 1cm 3.2cm 1cm},clip]{./figure/images/heatmap6_optimal_3000-n.pdf}
        \caption{Optimal}
        \label{figure:heatmap-oracle-app4}
    \end{subfigure}
    \begin{subfigure}{0.133\linewidth}
        \centering
            \includegraphics[width=0.98\linewidth, trim={3.2cm 1cm 3.2cm 1cm},clip]{./figure/images/heatmap6_RCUCB_500-n.pdf}
            \includegraphics[width=0.98\linewidth, trim={3.2cm 1cm 3.2cm 1cm},clip]{./figure/images/heatmap6_RCUCB_1500-n.pdf}
            \includegraphics[width=0.98\linewidth, trim={3.2cm 1cm 3.2cm 1cm},clip]{./figure/images/heatmap6_RCUCB_3000-n.pdf}
        \caption{CRUCB}
        \label{figure:heatmap-RCUCB-app4}
    \end{subfigure}
    \begin{subfigure}{0.133\linewidth}
        \centering
            \includegraphics[width=0.98\linewidth, trim={3.2cm 1cm 3.2cm 1cm},clip]{./figure/images/heatmap6_RUCB_500-n.pdf}
            \includegraphics[width=0.98\linewidth, trim={3.2cm 1cm 3.2cm 1cm},clip]{./figure/images/heatmap6_RUCB_1500-n.pdf}
            \includegraphics[width=0.98\linewidth, trim={3.2cm 1cm 3.2cm 1cm},clip]{./figure/images/heatmap6_RUCB_3000-n.pdf}
        \caption{R-ed-UCB}
        \label{figure:heatmap-RUCB-app4}
    \end{subfigure}
    \begin{subfigure}{0.133\linewidth}
        \centering
            \includegraphics[width=0.98\linewidth, trim={3.2cm 1cm 3.2cm 1cm},clip]{./figure/images/heatmap6_SWUCB_500-n.pdf}
            \includegraphics[width=0.98\linewidth, trim={3.2cm 1cm 3.2cm 1cm},clip]{./figure/images/heatmap6_SWUCB_1500-n.pdf}
            \includegraphics[width=0.98\linewidth, trim={3.2cm 1cm 3.2cm 1cm},clip]{./figure/images/heatmap6_SWUCB_3000-n.pdf}
        \caption{SW-UCB}
        \label{figure:heatmap-SWUCB-app4}
    \end{subfigure}
    \begin{subfigure}{0.133\linewidth}
        \centering
            \includegraphics[width=0.98\linewidth, trim={3.2cm 1cm 3.2cm 1cm},clip]{./figure/images/heatmap6_SWTS_500-n.pdf}
            \includegraphics[width=0.98\linewidth, trim={3.2cm 1cm 3.2cm 1cm},clip]{./figure/images/heatmap6_SWTS_1500-n.pdf}
            \includegraphics[width=0.98\linewidth, trim={3.2cm 1cm 3.2cm 1cm},clip]{./figure/images/heatmap6_SWTS_3000-n.pdf}
        \caption{SW-TS}
        \label{figure:heatmap-SWTS-app4}
    \end{subfigure}
    \begin{subfigure}{0.133\linewidth}
        \centering
            \includegraphics[width=0.98\linewidth, trim={3.2cm 1cm 3.2cm 1cm},clip]{./figure/images/heatmap6_CSWUCB_500-n.pdf}
            \includegraphics[width=0.98\linewidth, trim={3.2cm 1cm 3.2cm 1cm},clip]{./figure/images/heatmap6_CSWUCB_1500-n.pdf}
            \includegraphics[width=0.98\linewidth, trim={3.2cm 1cm 3.2cm 1cm},clip]{./figure/images/heatmap6_CSWUCB_3000-n.pdf}
        \caption{SW-CUCB}
        \label{figure:heatmap-SWCUCB-app4}
    \end{subfigure}
    \begin{subfigure}{0.133\linewidth}
        \centering
            \includegraphics[width=0.98\linewidth, trim={3.2cm 1cm 3.2cm 1cm},clip]{./figure/images/heatmap6_CSWTS_500-n.pdf}
            \includegraphics[width=0.98\linewidth, trim={3.2cm 1cm 3.2cm 1cm},clip]{./figure/images/heatmap6_CSWTS_1500-n.pdf}
            \includegraphics[width=0.98\linewidth, trim={3.2cm 1cm 3.2cm 1cm},clip]{./figure/images/heatmap6_CSWTS_3000-n.pdf}
        \caption{SW-CTS}
        \label{figure:heatmap-SWCTS-app4}
    \end{subfigure}
    
    \vspace{-0.1cm}
    % \caption{\textbf{Heatmap illustrating visit frequencies in AntMaze-complex.} 
    % We visualize the visit frequencies for the optimal policy, CRUCB, and baseline algorithms. 
    % The heatmap includes three rows representing visit frequencies until episode numbers 500, 1500, and 3000.
    % }
    \label{figure:heatmap-app4}
    \vspace{-0.3cm}
\end{figure}
